# Supplementary material for: Signature of lattice dynamics in twisted 2D homo/hetero-bilayers
Source: arXiv:2205.03497 source file (2022-05-06)
Supplement: Supplementary file 1 [file Supplementary_information.pdf]

# Supplementary information: Signature of lattice dynamics in twisted 2D homo/hetero-bilayers

Yang Pan<sup>1,2</sup>, Shutong Li<sup>3</sup>, Mahfujur Rahaman<sup>1,2\*</sup>, Ilya Milekhin<sup>1,2</sup>, and Dietrich R. T. Zahn<sup>1,2\*</sup>

<sup>1</sup>Semiconductor physics, Institut für Physik, Chemnitz University of Technology, Chemnitz, Germany

<sup>2</sup>Center for Materials, Architectures, and Integration of Nanomembranes (MAIN), Chemnitz University of Technology, Chemnitz, Germany

<sup>3</sup>Department of Chemical Engineering and Materials Science, University of Minnesota, Minneapolis, Minnesota, USA

\*Corresponding author: Dietrich R. T. Zahn: zahn@physik.tu-chemnitz.de  
Mahfujur Rahaman

## Sample preparation

### Preparation of twisted homo-bilayers:

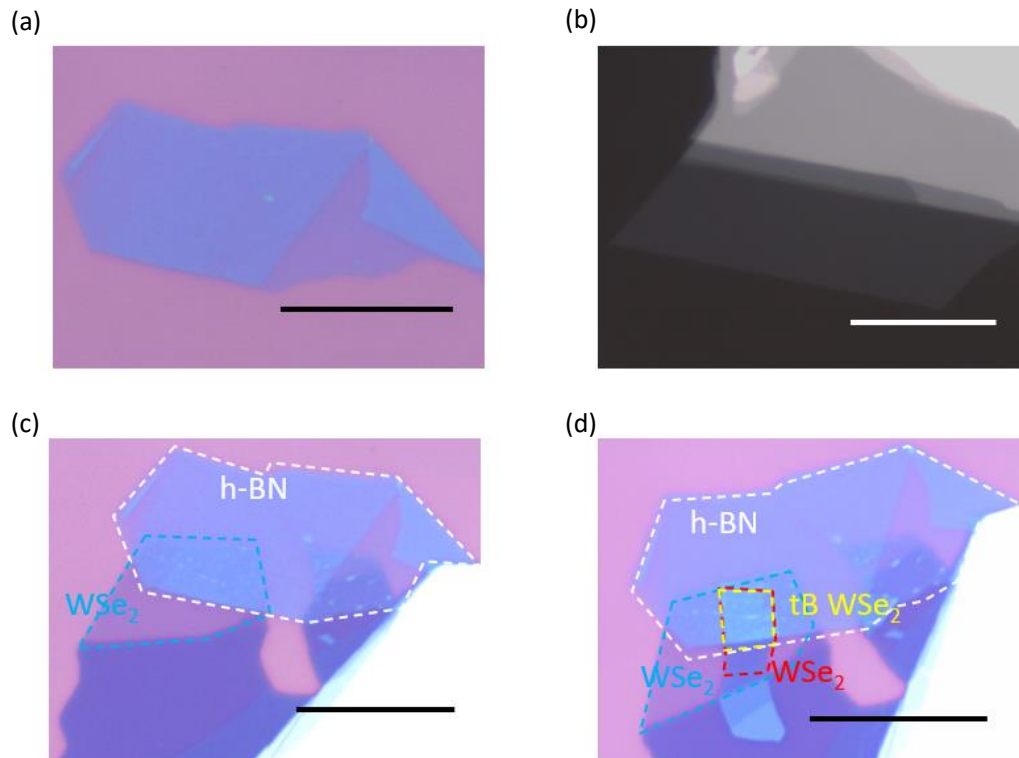

Figure S1. tB WSe<sub>2</sub> sample preparation. Optical image of (a) few layer hBN exfoliated on SiO<sub>2</sub> substrate, (b) monolayer WSe<sub>2</sub> exfoliated on PDMS, (c) partially transferred monolayer WSe<sub>2</sub> on hBN, and (d) tB WSe<sub>2</sub> on hBN. Scale bar is 20  $\mu\text{m}$ .

## Preparation of twisted hetero-bilayers

$30^\circ$  tB  $\text{WSe}_2$  is prepared following a tear-and-stack method. Due to the crystal symmetry, the breaking edges of these 2D materials can only be armchair or zigzag (shown in Fig. S2 (d)). A  $\text{MoSe}_2$  monolayer is later transferred on the  $30^\circ$  tB  $\text{WSe}_2$ , with one edge aligned to any  $\text{WSe}_2$  edge at an angle of  $30^\circ \times n$  ( $n$  is any integer number). This alignment results in 2 areas of heterostructures, one with a relative twisting angle of  $30^\circ$  and the other with  $0^\circ$  or  $60^\circ$ .

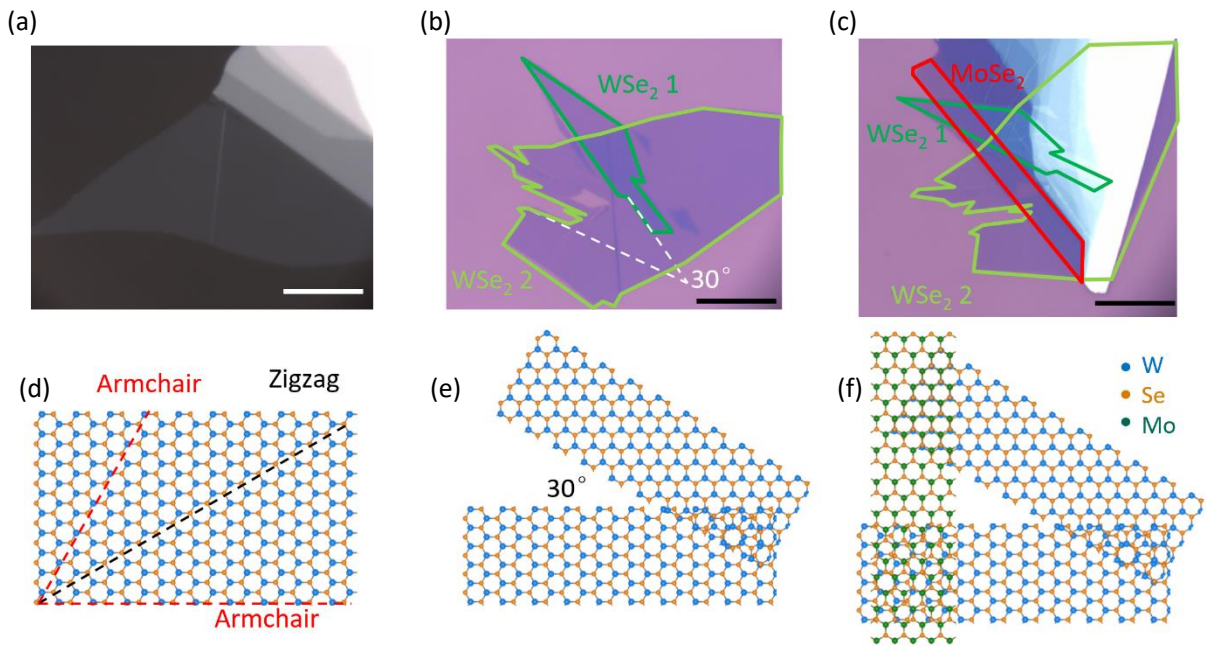

Figure S2. Twisted hetero-bilayer sample preparation. Optical image of (a) monolayer  $\text{WSe}_2$  exfoliated on PDMS, (b)  $30^\circ$  tB  $\text{WSe}_2$  on  $\text{SiO}_2$ , (c) twisted  $\text{MoSe}_2/\text{WSe}_2$  hetero-bilayer. (d)-(e) are the schematic crystal structures, respectively. Scalebar is  $10\ \mu\text{m}$ .

## Atomic structures for first-principles calculations

Bulk  $\text{WSe}_2$  is known to crystallize in the 2H structure. However, the artificial stacking of  $0^\circ$  and  $60^\circ$  twisted bilayer  $\text{WSe}_2$  can lead to at least 5 possible high symmetry atomic structures, as shown in Fig. S3.

First-principles calculations are performed for these high symmetry structures: the 2H, 3R phases at  $0^\circ$  and  $\text{AB}'$ ,  $\text{A}'\text{B}$ , 2H-phases at  $60^\circ$  to find the ground state structures.

A set of commensurate twisted bilayer  $\text{WSe}_2$  structures are also calculated with various numbers of atoms, including those with twisting angles of  $21.8^\circ$ ,  $27.8^\circ$  and  $38.2^\circ$ . These degrees are specifically selected in order to apply the periodic boundary condition.

It is found that the 2H phase at  $60^\circ$  and the 3R phase at  $0^\circ$  have the lowest energy as shown in Fig. S3. Thus, these two phases will be selected as unit cells for the simulations of  $0^\circ$  and  $60^\circ$  twisted bilayers. Structures at  $21.8^\circ$ ,  $27.8^\circ$  and  $38.2^\circ$  are also fully relaxed for the further simulations, using density functional theory. We pick these three data points because they are representative and close to  $30^\circ$ , although the demand for computational resources is very significant.

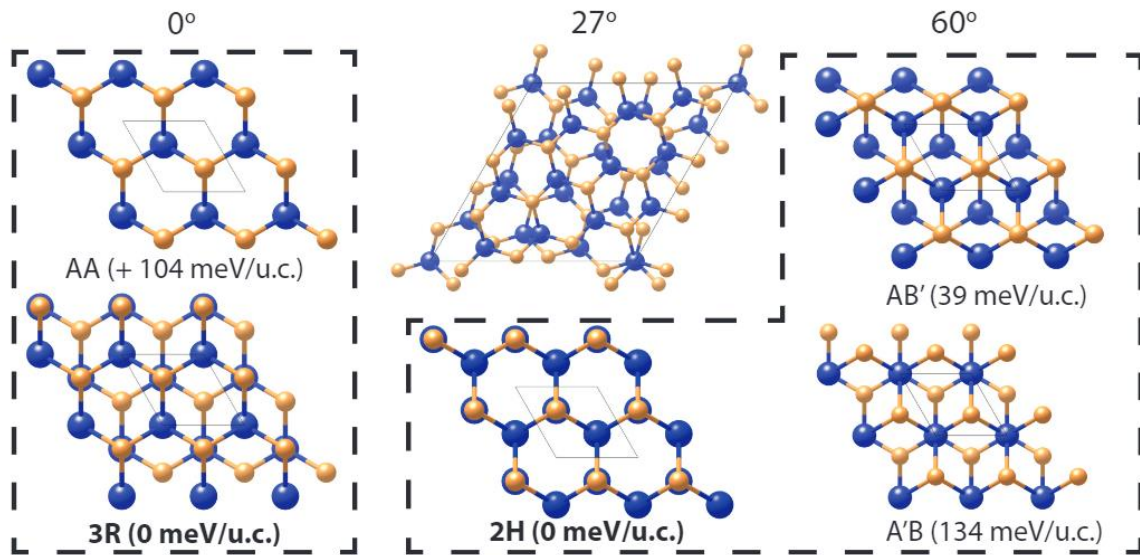

Figure S3. Possible structures of twisted bilayer  $\text{WSe}_2$ . The 3R phase has the lowest energy when the bilayer is untwisted. While at  $60^\circ$ , the 2H phase is the most stable one. Other possible crystal structures for  $0^\circ$  and  $60^\circ$  twisting angle are also shown in this plot, they are possibly observable when mechanically stacked. The commensurate crystal structures used for  $27^\circ$  twisting angle are also shown in the middle. The same calculations were also performed on  $21^\circ$  and  $38^\circ$  twisted structures.

## Raman spectra simulation

The simulation configurations are exactly the same as the ones used for structure relaxation. The calculated frequencies are listed in the main text Table 1. The phonon modes are extracted and later used for the Raman tensor calculation. The off-resonant Raman tensor can be calculated by the change of polarizability:

$$\tilde{R}_{\alpha\beta} \propto \frac{\Delta\varepsilon_{\alpha\beta}^{\infty}}{\Delta Q(s)} = \frac{1}{2} \left( -\frac{\varepsilon_{\alpha\beta}^{\infty}(-s)}{\Delta Q(s)} + \frac{\varepsilon_{\alpha\beta}^{\infty}(+s)}{\Delta Q(s)} \right)$$

where the  $\varepsilon$  stands for the ion-clamped dielectric constant, *i.e.* the dielectric constant at infinite high frequency. The  $Q(s)$  stands for the amplitude of normal mode  $s$  and  $\alpha, \beta$  indicate the directions. The normal mode  $s$  comes from the phonon calculation mentioned above. The derivative of them can be calculated by freezing in the phonon mode  $s$  in both positive and negative directions and calculate the change of dielectric constant then divided by the amplitudes.

We use the Perturbation Expression After Discretization (PEAD) method to determine the dielectric constant at infinity frequencies (which is the ion-clamped dielectric constant). This method is a self-consistent calculation under an applied electric field. The applied electric field was set to be 10 meV/Å.

Later on, the non-resonant Raman intensity can be determined by the Raman tensor:  $I_{Raman} \propto |\mathbf{e}_i \cdot \tilde{\mathbf{R}} \cdot \mathbf{e}_s|$ . The  $\mathbf{e}_i$  and  $\mathbf{e}_s$  are the polarization direction of incident and scattered light. In our experimental setup, the incident light is polarized to the in-plane direction. Both directions of in-plane scattered light were collected, which results in the total Raman intensity  $I \propto I_{xx} + I_{yy} \propto R_{xx}^2 + R_{yy}^2$ . Fig. S4 shows the calculated Raman spectra when the bilayer WSe<sub>2</sub> is twisted from 0° to 60°. The spectra in rectangular box are zoomed in by 100 times for visualization. However, compared to the experimental results, the B<sub>2g</sub> mode is weaker, which is likely due to the inability of capturing the resonant Raman intensity. It is reported that the B<sub>2g</sub> mode has resonant-Raman activity and can be observed even in some selection-rule prohibited structures<sup>1</sup>.

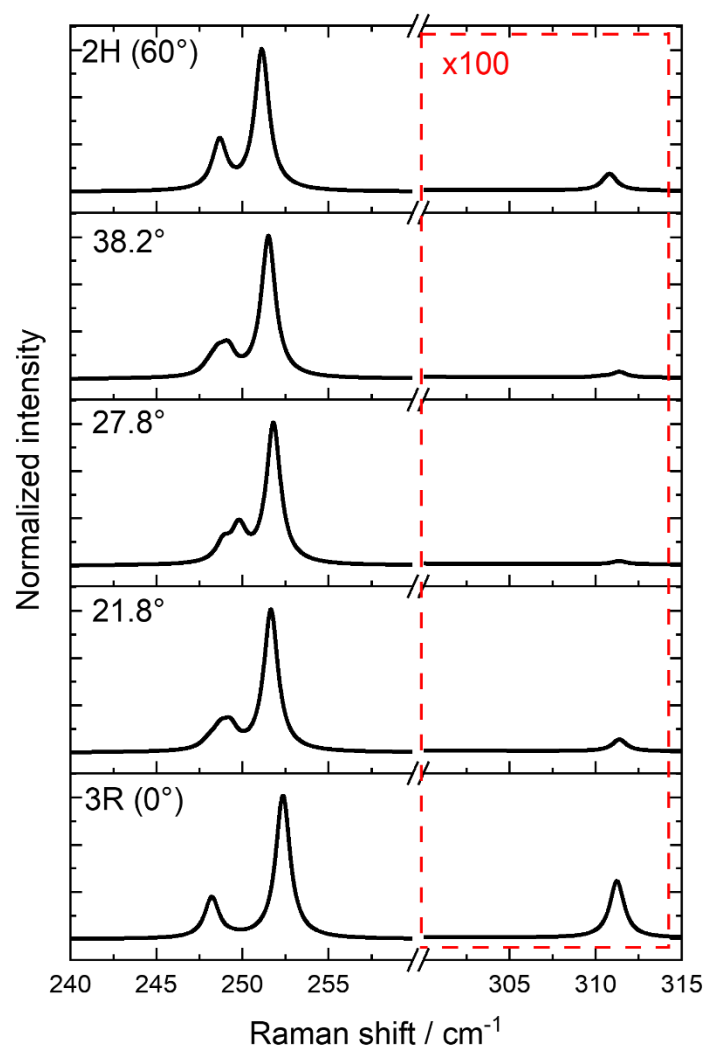

Figure S4. Simulated Raman spectra of 3R (0°), 21.8°, 27.8°, 38.2° and 2H (60°) bilayer WSe<sub>2</sub>. The spectra between 300 cm<sup>-1</sup> to 315 cm<sup>-1</sup> in the rectangular box are zoomed by 100 times for better visualization.

## Crystal structure in moiré superlattices

The structures of 2°, 5°, 10°, and 30° tB WSe<sub>2</sub> are shown in Fig. S5. The moiré superlattice constant is calculated with the equation<sup>2</sup>:

$$a_{\text{moiré}} = \frac{0.5a}{\sin(\theta/2)}$$

Where  $a$  is the in-plane lattice constant of WSe<sub>2</sub> and  $\theta$  is the twisting angle. The energy preferable AB and BA stacking area is absent in 30° tB WSe<sub>2</sub>.

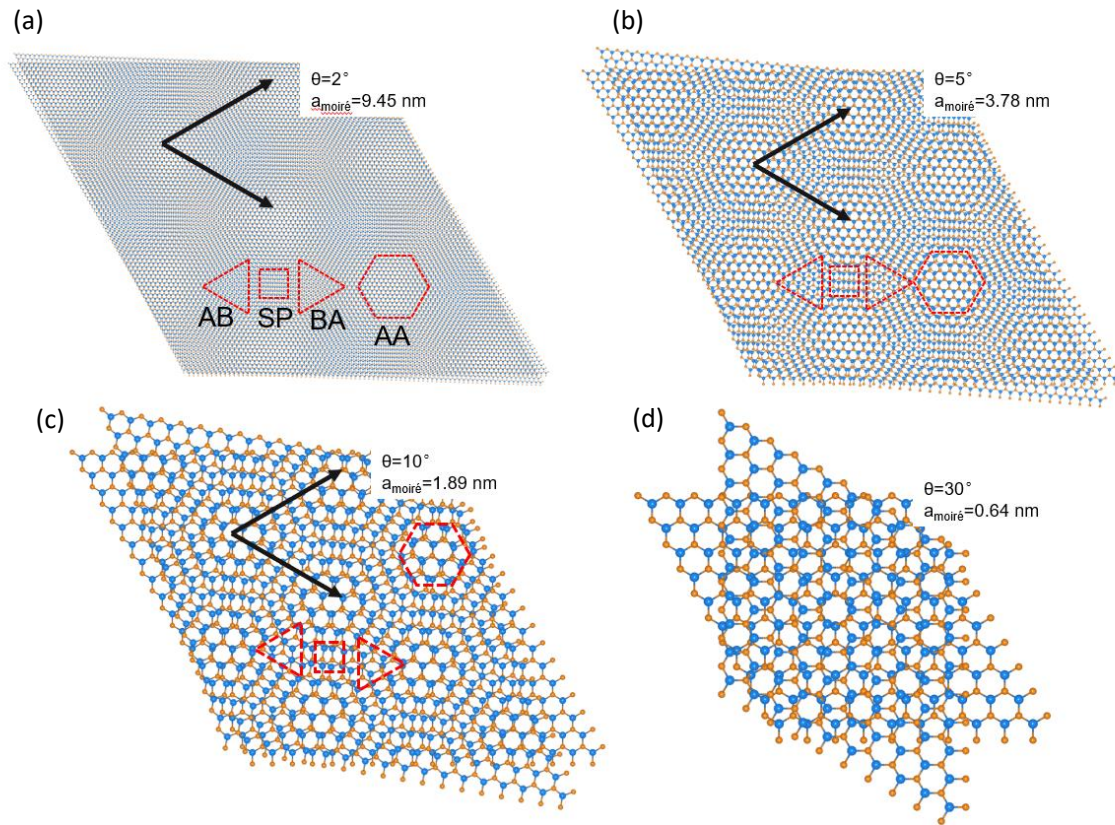

Figure S5. Schematic diagrams of WSe<sub>2</sub> moiré superlattices with different twisting angles: (a) 2°, (b) 5°, (c) 10°, and (d) 30°.

## Temperature-dependent Raman spectra of WSe<sub>2</sub>

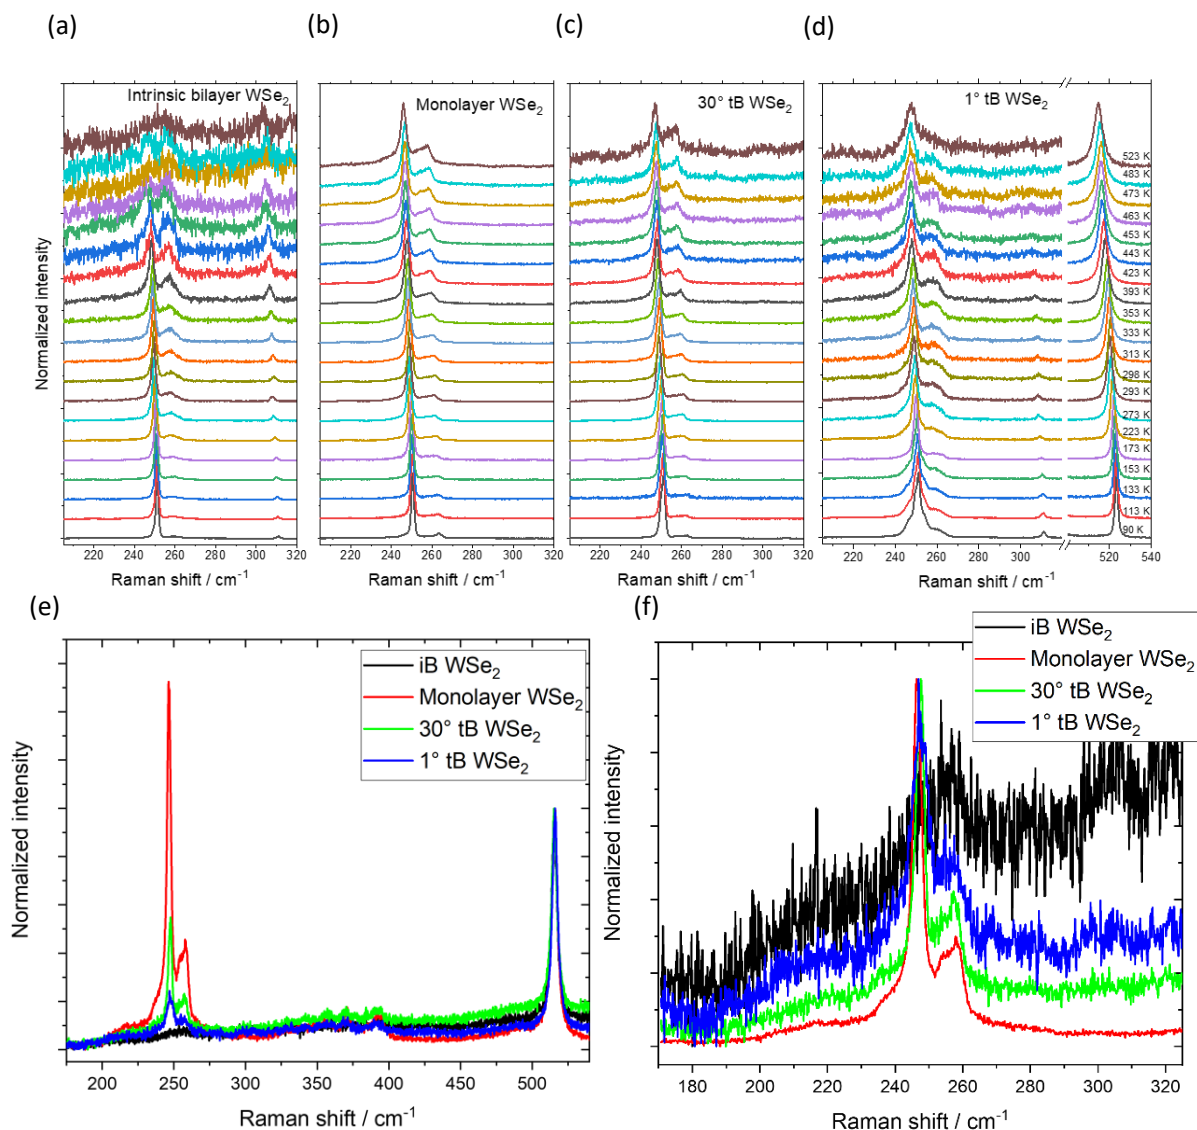

Figure S6. Temperature-dependent Raman spectra of (a) iB, (b) monolayer, (c) 30° tB WSe<sub>2</sub>, and (d) 1° tB WSe<sub>2</sub> with the silicon Raman peak used for temperature determination. Note that the Raman spectra in the ranges of 205- 320 cm<sup>-1</sup> and 500- 540 cm<sup>-1</sup> are normalized separately. (e) and (f) are the Raman spectra of iB, monolayer, 30° tB, and 1° tB WSe<sub>2</sub> at 473 K normalized with respect to the Si and WSe<sub>2</sub> E<sub>2g</sub>/A<sub>1g</sub> peaks, respectively.

Temperature-dependent Raman spectra of iB, monolayer, 30° and 1° tB WSe<sub>2</sub> are shown in Fig. S6 (a-d), respectively. The Raman signal of iB WSe<sub>2</sub> is almost not visible when the temperature is higher than 473 K, while monolayer and 30° tB WSe<sub>2</sub> behave completely differently from the iB case, whereas 30° tB WSe<sub>2</sub> has similar behavior as monolayer. The Raman signal of 1° tB WSe<sub>2</sub> is still visible at high temperature. However, as shown in Fig. S6 (e) and (f), it has much lower intensity and signal-to-noise ratio compared to monolayer and 30° tB WSe<sub>2</sub>, which can be explained by relatively weaker interlayer coupling because of the existence of non-AA/AB stacking area and hydrocarbonate contamination at the interface due to the artificial stacking.

The temperature dependent Raman spectra of Si are also plotted in Fig. S6(d). With increasing temperature, the Si Raman feature shifts towards lower frequency and shows a broadening of the FWHM, which is in good agreement with previous studies<sup>3,4</sup>. The temperature dependence of the Si Raman peak can be used as an indicator of the temperature.

## Temperature-dependent PL spectra and Varshni's plot

Temperature-dependent PL spectra of iB, monolayer, and 30° tB WSe<sub>2</sub> are shown in Fig. S7 (a-c). The 30° tB WSe<sub>2</sub> has a similar PL response as the monolayer WSe<sub>2</sub>, while there is a huge difference to that of iB WSe<sub>2</sub>. The direct transition PL peak position is plotted in Fig (d-e) and fitted with the modified Varshni's equation<sup>5-8</sup>:

$$E_g(T) = E_g(0) - S\langle\hbar\omega\rangle \left[ \coth\left(\frac{\langle\hbar\omega\rangle}{2k_B T}\right) - 1 \right]$$

Where  $E_g(0)$  is the transition energy at T=0 K,  $S$  is a dimensionless constant that describes the strength of electron-phonon coupling, and  $\langle\hbar\omega\rangle$  describes the average acoustic phonon energy involved in electron-phonon interactions.

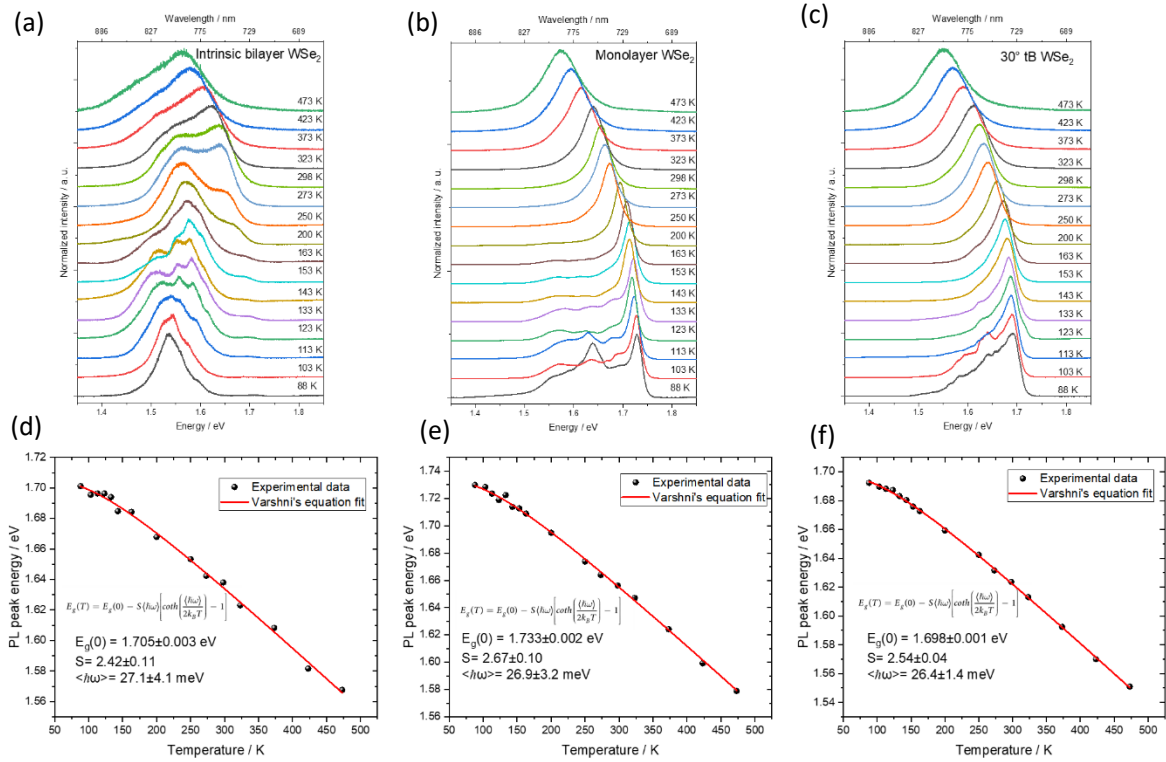

Figure S7. Temperature dependent Raman spectra of (a) iB, (b) monolayer, (c) 30° tB WSe<sub>2</sub> and the corresponding A exciton positions fitted with Varshni's equation (d)-(f).

# Raman map of twisted hetero-bilayers

We further investigated different combination of TDMCs. Both  $\text{WSe}_2/\text{MoS}_2$  and  $\text{MoSe}_2/\text{WSe}_2$  hetero-bilayers show consistent results as in main text. One can clearly identify the contrast between the two areas with different crystal orientations in the Raman intensity ratio map.

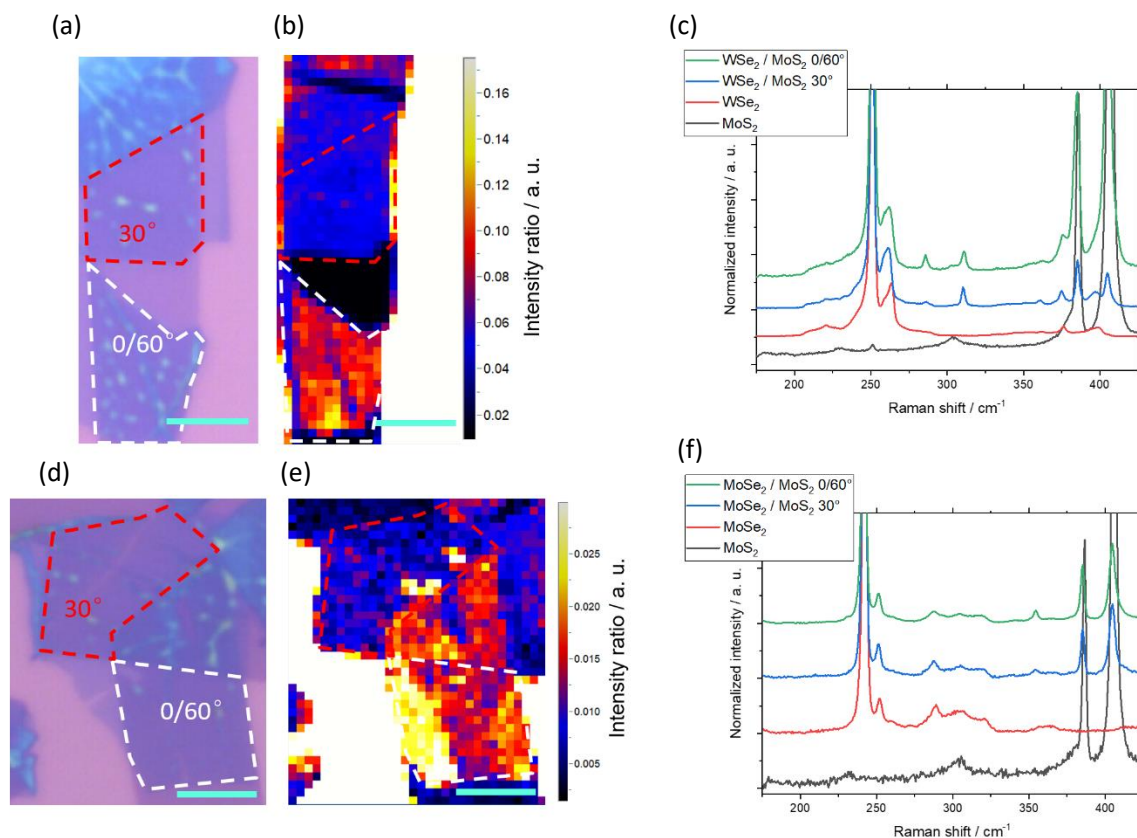

Figure S8. Raman maps of twisted hetero-bilayers. Optical image of twisted (a)  $\text{WSe}_2/\text{MoS}_2$  (d)  $\text{MoSe}_2/\text{WSe}_2$ , areas marked by red and white dashed lines have twisting angles of 30° and 0/60°, respectively. Raman intensity ratio maps of (b)  $\text{WSe}_2$   $I_{B_{2g}}/I_{E_{2g} A_{1g}}$  and (e)  $\text{MoSe}_2$   $I_{B_{2g}}/I_{A_{1g}}$ . Corresponding Raman spectra normalized to (c)  $\text{WSe}_2$   $E_{2g}/A_{1g}$  and (f)  $\text{MoSe}_2$   $A_{1g}$ . Scalebar is 5  $\mu\text{m}$ .

## References

1. Luo, X. *et al.* Effects of lower symmetry and dimensionality on Raman spectra in two-dimensional  $\text{WSe}_2$ . *Phys. Rev. B - Condens. Matter Mater. Phys.* **88**, 1–7 (2013).
2. Moon, P. & Koshino, M. Optical absorption in twisted bilayer graphene. *Phys. Rev. B - Condens. Matter Mater. Phys.* **87**, 1–11 (2013).
3. Tsu, R. & Hernandez, J. G. Temperature dependence of silicon Raman lines. *Appl. Phys. Lett.* **41**, 1016–1018 (1982).
4. Hart, T. R., Aggarwal, R. L. & Lax, B. Temperature dependence of raman scattering in silicon. *Phys. Rev. B* **1**, 638–642 (1970).

5. Huang, J., Hoang, T. B. & Mikkelsen, M. H. Probing the origin of excitonic states in monolayer WSe<sub>2</sub>. *Sci. Rep.* **6**, 1–7 (2016).
6. Ross, J. S. *et al.* Electrical control of neutral and charged excitons in a monolayer semiconductor. *Nat. Commun.* **4**, 1–6 (2013).
7. Tongay, S. *et al.* Thermally driven crossover from indirect toward direct bandgap in 2D Semiconductors: MoSe<sub>2</sub> versus MoS<sub>2</sub>. *Nano Lett.* **12**, 5576–5580 (2012).
8. O'Donnell, K. P. & Chen, X. Temperature dependence of semiconductor band gaps. *Appl. Phys. Lett.* **58**, 2924–2926 (1991).
